# Supplementary material for: LoRA and Privacy: When Random Projections Help (and When They Don't)
Source: arXiv:2601.21719 source file (2026-01-29)
Supplement: Supplementary file 1 [file conv_analysis_vecproj.tex]

In this section, we analyse the convergence guarantee of projection mechanism when applied to convex optimization problem. We show that under the minimum alignment assumption between the dataset collection $\cD$ and the gradient trajectory $f$, gradient descent with projection mechanism (RP-GD) achieves a convergence rate comparable to, and in some regimes better than, that of DP-GD for smooth convex optimization. 

For a dataset $S = \{(x_i, y_i)\}_{i = 1}^n$, let $\ell:\cW \times (\cX\times \cY) \to \bR_+$ be a loss function. Then, let $\cL:\cW \times \cZ \to \bR_+ $ be the loss function over the entire dataset, i.e. $\cL(w; S)= \frac{1}{n}\sum_{i = 1}^n \ell(w, (x_i, y_i))$. The optimization problem is defined in~\Cref{eq:optimization-object}. 
\begin{equation}
    \label{eq:optimization-object}
    \hat{w} = \text{arg}\min_{w\in \cW} \frac{1}{n} \sum_{i = 1}^n \ell(w, x_i, y_i) =: \text{arg}\min_{w\in \cW} \cL(w; S).
\end{equation}

The most common private approach is DP-GD (equivalently, Noisy-GD when there is no gradient clipping), which attains a convergence rate of $\sqrt{d}/(T\varepsilon)$ \citep{Abadi2016,bassily2014}. At each step, DP-GD applies the Gaussian mechanism (\Cref{defn:gaussian-mech}) to the gradient and then performs a gradient-descent update with the noisy gradient. In contrast, we propose \emph{Randomly Projected Gradient Descent (RP-GD)}: first apply the projection mechanism (\Cref{defn:projection-mech}) to the gradient, then take a gradient descent step with the projected output. Specifically, sample $M \sim \mathsf{W}_d(\sigma^2 I_d, r)$ once and update at each time step with the following update function, 
\begin{equation}
    \label{eq:rp-gd-update}
    w_{t+1} = w_t - \eta M \nabla \cL(w_t).
\end{equation}

RP-GD enjoys the following convergence guarantee. 
\begin{restatable}{thm}{ConvexSmoothConvergence}\label{thm:convergence-convex-smooth}
    For a dataset collection $\cD$ and the query function $f(w_0, S) = \sum_{i = 0}^T\nabla \cL(w_i; S)$, let the minimum alignment of $f$ on $\cD$ be $\rho$. For any dataset $S\in \cD$, if $d \leq \frac{3}{4}r$, $r\geq 16\log \frac{1}{\delta}$ and assume $\cL$ is convex and $\beta$-smooth, then RP-GD is $(\epsilon_\rho, \delta)$-DP where $\epsilon_\rho = Cr\sqrt{1-\rho}/\rho$ for some constant $C$ independent of $d, r$, and with probability at least $1-2\delta$, 
    \[\cL(w_T) - \cL_S^\star =O\br{ \frac{\beta\norm{w_0 -w_S^\star}_2}{2T}}\]
    where $w_S^\star = \argmin \cL(w; S)$ and $\cL_S^\star = \min \cL(w; S)$. 
\end{restatable}

Our bound improves upon DP-GD when the dataset collection has well-aligned gradient sums. In
particular, when the minimum alignment is large (e.g., \(\rho = \tfrac{r}{r+1}\)), the privacy
parameter \(\epsilon\) remains a constant, and RP-GD achieves an \(O(1/T)\) convergence rate that
is independent of the dimension \(d\). By contrast, if we fix \(\epsilon=C\), then DP-GD converges
at rate \(O(\sqrt{d}/T)\). For less aligned datasets, for example, when \(0<\rho<0.5\), we obtain
\(\epsilon = O(d)\), and the convergence guarantee of RP-GD is comparable to that of DP-SGD.

If the minimum-alignment assumption does not hold for the cumulative gradient over \(T\) steps, we
can relax it by requiring alignment only at the per-step gradient level and resampling a new
projection at each step. This relaxation incurs an additional factor of \(T\) in the privacy
guarantee due to composition across steps. Notably, when \(r \le d\), this procedure coincides with
CompSGD~\citep{kasiviswanathan21a}, which also achieves nearly dimension-independent convergence
guarantees.

\textbf{Low-rank version also saves space and computation} We note that~\Cref{eq:rp-gd-update} is equivalent to first performing a gradient descent in random projected subspaces using a variable $z_0 = Z w_0\in \bR^r$ and the projection matrix $Z \in \bR^{d\times r}$ where $M = ZZ^\top$, by parameterizing $w_t = w_t + Z^\top z_t$ \citep{Hao2024Flora}. Therefore, when $r < d$, RP-GD is also more computationally and memory efficient. 
\as{Don't need both here }

\ConvexSmoothConvergence*
\begin{proof}
    \textbf{Convergence:} For a dataset $S\in \cD$, condition on a projection matrix $M$ with $\lambda_{max}(M) > 0$ and $\lambda_{\min}(M) > 0$. We first show that $\cL(w_T) - \cL_S^\star \leq \frac{\beta \lambda_{\max}\norm{w_0 - w_S^\star}_2}{T\lambda_{\min}}$.

    Let $v_t = \nabla \cL(w_t)$. By smoothness of $\cL$, 
    \begin{equation}
        \label{eq:smoothness-convergence-convex}
        \begin{aligned}
        \cL(w_{t+1})&\leq \cL(w_t) - \eta v_t^\top M v_t + \frac{\beta \eta^2}{2}\norm{M v_t}^2\\
        &\leq \cL(w_t) - \eta v_t^\top M v_t + \frac{\beta \eta^2}{2}\lambda_{\max}v_t^\top  Mv_t \\ 
        &\leq \cL(w_t) - \eta\br{1 - \frac{\beta\eta\lambda_{\max}}{2}}v_t^\top Mv_t\\
        &\leq \cL(w_t) - \frac{\eta}{2}v_t^\top Mv_t
        \end{aligned} 
    \end{equation}
    where the last inequality follows by $\eta \leq \frac{1}{2\beta \lambda_{\max}}$. 
    Rearranging, \begin{equation}
        \label{eq:smoothness}
        v_t^\top M v_t \leq \frac{2}{\eta}\br{\cL(w_t) - \cL(w_{t+1})}
    \end{equation}
    Then 
    \begin{equation}
        \begin{aligned}
            \norm{w_{t + 1}-w_S^\star}_{M^{\dagger}}^2 &= (w_{t + 1}-w_S^\star)^\top M^{\dagger} (w_{t + 1}-w_S^\star)\\
            &= (w_{t}-w_S^\star-\eta Mv_t)^\top M^{\dagger} (w_{t}-w_S^\star-\eta Mv_t)\\
            &= (w_t-w_S^\star)^\top M^{\dagger} (w_t-w_S^\star) - 2\eta v_t^\top MM^{{\dagger}} (w_t-w_S^\star)  + \eta^2 v_t^\top M v_t\\
            &=\norm{w_t-w_S^\star}_{M^{\dagger}} -2\eta v_t^\top   (w_t-w_S^\star) - 2\eta v_t^\top (MM^{{\dagger}} - I)  (w_t-w_S^\star)+ \eta^2 v_t^\top M v_t.
        \end{aligned}
    \end{equation}

    By convexity of $\cL$, 
    \[\cL(w_t) - \cL(w_S^\star)\leq v_t^\top (w_t-w_S^\star)\]

    Therefore, by convexity and~\Cref{eq:smoothness}
     \begin{equation}
        \begin{aligned}
            \norm{w_{t + 1}-w_S^\star}_{M^{-1}}^2 &\leq \norm{w_t-w_S^\star}_{M^{-1}} - 2\eta \br{\cL(w_t) - \cL(w_S^\star)}  + 2\eta  \br{\cL(w_t) - \cL(w_{t+1})} - 2\eta v_t^\top (MM^{{\dagger}} - I)  (w_t-w_S^\star)\\
            &= \norm{w_t-w_S^\star}_{M^{-1}} + 2\eta \br{\cL(w_S^\star)-\cL(w_{t+1})} + 2\eta v_t^\top (I-MM^{{\dagger}} )  (w_t-w_S^\star)
        \end{aligned}
    \end{equation}
    Rearrange, 
    \begin{equation}\label{eq:before-telescoping}
        \cL(w_{t+1}) - \cL(w_S^\star)\leq \frac{1}{2\eta}\br{ \norm{w_t-w_S^\star}_{M^{-1}}  - \norm{w_{t + 1}-w_S^\star}_{M^{-1}}^2 }+v_t^\top (M^{\dagger} M - I) (w_0 - w_S^\star)
    \end{equation}
    where the last part follows by $w_t = w_0 + M\sum_{i = 1}^t \eta v_t$ and $(M^{\dagger} M - I)M = 0$. 
    
    As $\cL(w_t)$ is monotonically decreasing~(\Cref{eq:smoothness}), 
    \begin{equation}
    \begin{aligned}
        \cL(w_T) - \cL(w_S^\star) &\leq \frac{1}{T}\sum_{t = 1}^T \cL(w_t) - \cL(w_S^\star) \\
        &\leq \frac{1}{2\eta T}\sum_{t = 1}^T\norm{w_t-w_S^\star}_{M^{-1}}  - \norm{w_{t + 1}-w_S^\star}_{M^{\dagger}}^2 +\frac{1}{T}\sum_{i = 1}^T v_t^\top (M^{\dagger} M - I)(w_0 - w_S^\star)&&\because\Cref{eq:before-telescoping}\\
        &\leq \frac{\norm{w_0 - w^\star_S}_{M^{\dagger}}}{2\eta T} \leq \frac{ \norm{w_0 - w^\star_S}\lambda_{\max}(M) }{2T\lambda_{\min}(M)}
    \end{aligned}
    \end{equation}

    By initializing $w_0\sim \cN(0, I_d/(dT))$, the first term $\norm{(M^{\dagger} M - I)w_0} =O\br{ \frac{1}{Td}}$ with high probability. 
    (Variance $\sigma^2$ cancels out; CHECK) 
    By~\Cref{lem:singular-value-lower-tail} and~\Cref{lem:gaussian-random-matrices-tails}, for some $t, t'$, and for $M = \sigma^2 ZZ^\top$ where $Z\in \bR^{d\times r}$ with each entry i.i.d. standard Gaussian
    \[\bP(\lambda_{\max}(M) > \sigma^2(\sqrt{d} + \sqrt{r} + t)^2 ) = \bP(\lambda_{\max}(Z) > \sqrt{d} + \sqrt{r} + t ) \leq e^{-\frac{t^2}{2}}\]
    Setting $t = \sqrt{2\log\frac{1}{\varsigma}}$, we have \begin{equation*}
        \bP\bs{\lambda_{\max}(M) > \br{\sqrt{d} + \sqrt{r} + \sqrt{2 \log\frac{1}{\varsigma}}}^2 } \leq \varsigma
    \end{equation*}
    As $r \geq 3d/4$, 
    \begin{equation}
        \label{eq:convergence-prob-1}
        \begin{aligned}
             \bP\bs{\lambda_{\max}(M) > \sigma^2\br{2\sqrt{r}  + \sqrt{2\log\frac{1}{\varsigma}}}^2 }&\leq \bP\bs{\lambda_{\max}(M) > \sigma^2\br{\br{1 + \frac{\sqrt{3}}{2}}\sqrt{r}  + \sqrt{2\log\frac{1}{\varsigma}}}^2 }\\
             &\leq \bP\bs{\lambda_{\max}(M) > \sigma^2\br{\sqrt{d} + \sqrt{r} + \sqrt{2\log\frac{1}{\varsigma}}}^2 } \leq \varsigma
        \end{aligned}
    \end{equation}
    Similarly, 
    \begin{equation}
        \label{eq:convergence-prob-2}
        \bP\bs{\lambda_{\min}(M) < \sigma^2\br{\frac{1}{2}\sqrt{r}- \sqrt{2\log\frac{1}{\varsigma}}}^2}\leq \bP\bs{\lambda_{\min}(M) < \sigma^2\br{\sqrt{r} - \sqrt{d} - \sqrt{2\log\frac{1}{\varsigma}}}^2 } \leq \varsigma
    \end{equation}
    Condition on these two events, which occur with probability at least $1-2\varsigma$, we substitute in $\lambda_{\max} \leq \sigma^2\br{2\sqrt{r}  + \sqrt{2\log\frac{1}{\varsigma}}}^2$ and $\lambda_{\min} \geq 
    \sigma^2\br{\frac{1}{2}\sqrt{r}- \sqrt{2\log\frac{1}{\varsigma}}}^2 $, which yields the desired result. 
\end{proof}

\begin{restatable}{thm}{NaiveConvergence}\label{thm:convergence-smooth}
    Let $F$ be $\beta$-smooth. Let $x_1, ..., x_T$ be the outputs produced by RP-GD with update function~(\Cref{eq:rp-gd-update}). Then, $x_1, ..., x_T$ satisfies \[\bE\bs{\frac{1}{T}\sum_{t = 1}^T \norm{\nabla F(x_t)}} \leq \sqrt{\frac{2\beta \br{ 1 + \frac{d  +1}{r}}\br{F(x_0) - F(x^\star)}}{T}},\]
    where the randomness is over all projection matrices $P_1, ..., P_T$. 
\end{restatable}
% \NaiveConvergence*
\begin{proof}
    Assume $F = \frac{1}{n}\sum_{i = 1}^n f_i$ is $\beta$-smooth, then \[F(x + h) \leq F(x) + \ba{\nabla F(x), h} + \frac{\beta}{2}\norm{h}^2. \]
    For notational simplicity, we write $g_t = \frac{\nabla F(x_t)}{\norm{\nabla F(x_t)}}$. Following the update rule of RP-GD~(\Cref{eq:rp-gd-update}) and by the smoothness of $F$, for any $P_t\in \bR^{d\times r}$, 
    \begin{equation*}
    \begin{aligned}
                F(x_{t+1}) &\leq F(x_{t}) - \eta\ba{\nabla F(x_{t}), P_t P_t^\top\nabla \frac{F(x_{t})}{\norm{F(x_{t})}} } + \frac{\eta^2\beta}{2}\norm{P_t P_t^\top \frac{\nabla F(x_{t})}{\norm{\nabla F(x_{t})}}}^2 \\
                &= F(x_{t}) - \norm{\nabla F(x_t)} \ba{g_t, -\eta P_t P_t^\top g_t} + \frac{\beta \eta^2}{2} \norm{P_t P_t^\top g_t}^2\\
                &= F(x_t) - \eta \norm{\nabla F(x_t)} \norm{P_t^\top g_t}^2 + \frac{\beta\eta^2}{2}\norm{P_t P_t^\top g_t}^2
    \end{aligned}
    \end{equation*}
    Rearranging the above equation, 
    \begin{equation}
        \label{eq:convergence-1}
        \norm{\nabla F(x_t)} \norm{P_t g_t}^2 \leq \frac{F(x_t) - F(x_{t+1})}{\eta} + \frac{\beta\eta}{2}\norm{P_t^\top P_t g_t}^2
    \end{equation}
    By properties of Wishart distribution ($P_t^\top P_t\sim \sigma^2\text{Wishart}_d(m, I_d)$) (TODO: write the lemma), \[\bE_{P_t}\bs{\norm{P_t^T g_t}^2} = \bE_{P_t}\ba{g_t, P_t P_t^T g_t} = g_t^\top \bE_{P_t}\bs{P_t P_t^\top}g_t = r\sigma^2,\]
    \[\bE_{P_t}\bs{\norm{P_t P_t^\top g_t}^2} = \sigma^4 r(d + r+1) \]
    Where the they follows by~\Cref{lem:wishart-moments}. 
    
    Thus, conditional on all previous $P_\tau$, $\tau < t$ and taking expectation over $P_t$, 
    \[\norm{\nabla F(x_t)} \leq \frac{1}{\sigma^2 r}\bE_{P_t}\bs{\frac{F(x_t) - F(x_{t+1})}{\eta}|P_{1:t-1}} + \frac{\beta\eta\sigma^2 ( d+ r)}{2}.\]
    Summing over all $t$ and taking expectations over all $P_0, ..., P_T$, 
    \begin{equation}
        \bE\bs{\frac{1}{T}\sum_{t = 1}^T \norm{\nabla F(x_t)}} \leq \frac{1}{Tr\sigma^2}\bE\bs{\frac{F(x_0) - F(x_T)}{\eta}} + \frac{\beta \eta \sigma^2 ( d+ r)}{2} \leq \frac{F(x_0) - F(x^\star)}{Tr\sigma^2\eta} + \frac{\beta \eta \sigma^2 ( d+ r) }{2} 
    \end{equation}
    where $x^\star = \argmin_{x\in \cX} F(x)$. 

    Choosing $\eta^\star = \frac{1}{\sigma^2}\sqrt{\frac{2(F(x_0) - F(x^\star))}{\beta Tr(d + r)}}$, we get desired bound, 
    \[\bE\bs{\frac{1}{T}\sum_{t = 1}^T \norm{\nabla F(x_t)}} \leq \sqrt{\frac{2\beta \br{d+r}\br{F(x_0) - F(x^\star)}}{rT}}.\]
\end{proof}
