# Supplementary material for: LoRA and Privacy: When Random Projections Help (and When They Don't)
Source: arXiv:2601.21719 source file (2026-01-29)
Supplement: Supplementary file 2 [file miscellaneous.tex]

\begin{lem}\label{lem:upper-bound-sum-of-corr-biv}
    For $X_i$ and $Y_i$ standard bivariate random variables with correlation $\rho > 0$
    \[
        \mathbb{P}(\sum_{i=1}^r X_i Y_i < 0) \leq ( 1 - \rho^2 )^{r/2}
    \]
\end{lem}
\begin{proof}
    \begin{align}
        \mathbb{E}[e^{\lambda X_i Y_i}] = (1 - 2 \rho \lambda - (1- \rho^2)\lambda^2)^{-1/2} \text{ for } \lambda \in \left(- \frac{1}{1 - \rho}, \frac{1}{1 + \rho}\right) \text{ (write out proof as extra lemma) } \label{eq:mult-moment-bound}
    \end{align}
    in order to use this identity we will first convert the random variables to positive (exponential) random variables (multiply with $-t$ for $t>0$ and take exponential) and then apply~\Cref{eq:mult-moment-bound}:
    \[ 
        \mathbb{P}(\sum_{i=1}^r X_i Y_i < 0) = \mathbb{P}(e^{-t\sum_{i=1}^r X_i Y_i} \geq  1) \leq \mathbb{E}[ e^{-t\sum_{i=1}^r X_i Y_i}] = \prod_{i=1}^r
        \mathbb{E}( e^{-t X_i Y_i}  \geq 1) = (1 + 2 \rho t - (1 - \rho^2)t^2)^{-r/2}
    \]
    where we used the above identity with $\lambda = -t$. Now we want to find $t>0$ so that $q(t)^{-r/2}$ is minimized, with $q(t) = 1 + 2 \rho t - (1 - \rho^2)t^2$. As $ x \to x^{-r/2}$ is decreasing on $(0, \infty)$ this is equivalent to maximizing $q(t)$. 
    \begin{align*}
        q'(t) &= 2 \rho - 2(1 - \rho^2)t \\
        q''(t) &= - 2(1 - \rho^2) < 0
    \end{align*}
    so $t^* = \frac{\rho}{1 - \rho^2}$ maximizes $q(t)$. We remark here that $t^* = -\lambda$, so we need to check if $t^* \in (0, \frac{1}{1 - \rho})$ in order to be allowed to use~\Cref{eq:mult-moment-bound}. Which is indeed true as 
    \[
        \frac{\rho}{1 - \rho^2} < \frac{1}{1 - \rho} \iff \rho < 1 + \rho
    \]
    which is always true. So finally plugging this in we get:
    \begin{align*}
        q(t^*)  &= 1 + \frac{2 \rho^2}{1 - \rho^2} - \frac{(1 - \rho^2) \rho^2}{(1- \rho^2)^2} \\ 
                &= 1 + \frac{2 \rho^2}{1 - \rho^2} - \frac{\rho^2}{(1 - \rho^2)} = 1 + \frac{\rho^2}{1 - \rho^2} \\
                &= \frac{1}{1 - \rho^2}
    \end{align*}
    Finally plugging this into the bound we get the wished results.
\end{proof}

\begin{align*}
    W_T   &= W_0 - \eta \left( \sum_{t=1}^T \nabla_W \mathcal{L} + \sigma' E' \right) A_t^\top A_t     \\
    &=  W_0 - \eta \left( \sum_{t=1}^T \nabla_W \mathcal{L} A_t^\top + \sigma' E' A_t^\top \right) A_t \\
    & = W_0 - \eta \left( \sum_{t=1}^T \nabla_B\mathcal{L} + \sigma' E' A_t^\top \right) A_t 
\end{align*}

\jd{
I believe the last equality doesn't hold up because I believe: $\nabla_B\mathcal{L}|_{B= B_t} =  \nabla_W\mathcal{L}|_{W = W_t} A_{t-1}^\top$ . And this means we would have $\nabla_B\mathcal{L}|_{B= B_t} A_t = \nabla_W\mathcal{L}|_{W = W_t} A_{t-1}^\top A_t$
}

However what about the next update? The new weight matrix used for the forward pass would now be $W = W_0 + B_1 A = W_0$ and therefore dependent on $A$. We resolve this by resampling $A$:
\[
\begin{aligned}
    W_1 &= W_0 + B_1 A_0 \\
    \tilde{G} &= (\nabla_{W}\mathcal{L}(W_1;\mathcal{B}_t) + noise) \,A_1^\top A_1 \text{ where $A_1$ is resampled} \\
    W_2 &= W_1 - G
\end{aligned} 
\]

\begin{algorithm}[h]
\caption{Noisy Projection Mechanism with resampling ($T$ steps, one layer)}
\label{algo:noisy-proj-mech-resample}
\textbf{Input:} pretrained $W_0\in\mathbb{R}^{n\times d}$; rank $r$; steps $T$; step size $\eta$;
dataset size $N$; minibatch size $B_{\mathrm{mb}}$; loss $\mathcal L$;
clipping level $\beta'$; privacy parameters $(\varepsilon,\delta)$.\\
\textbf{Notation:} $\mathrm{clip}_{\beta'}(X)=\min\!\left(1,\frac{\beta'}{\|X\|_F}\right)X$.
\begin{algorithmic}
  \STATE \textbf{Initialize} $B \gets 0 \in \mathbb{R}^{n\times r}$.
  \STATE \textbf{Sample} $A_0 \sim \mathcal N(0,1/\sqrt{r})^{r\times d}$.
  \STATE $W_1 = W_0 + BA_0$
  \FOR{$t=1,\dots,T$}
    \STATE Sample minibatch $\mathcal{B}_t\subset[N]$ with $|\mathcal{B}_t|=B_{\mathrm{mb}}$ (or take $\mathcal{B}_t=[N]$).
    % \STATE \textbf{Forward weights (use previous projection):} $W_t \gets W_0 + BA_{t-1}$.
    \STATE Compute gradient $G_t \gets \nabla_W \mathcal L(W_t;\mathcal{B}_t)\in\mathbb{R}^{n\times d}$.
    \STATE \textbf{Resample projection for the private release:} sample $A_t \sim \mathcal N(0,1/\sqrt{r})^{r\times d}$.
    \STATE \textbf{Noisy projected update:}
    $\widehat G_t \gets \bigl(\mathrm{clip}_{\beta'}(G_t)+\sigma' E_t\bigr)\,A_t^\top A_t$,
    where $(E_t)_{ij}\overset{\mathrm{i.i.d.}}{\sim}\mathcal N(0,1)$.
    % \STATE \textbf{Update} $B \gets B - \eta\,\widehat U_t\,A_{t-1}^\top\,(A_{t-1}A_{t-1}^\top)^{-1}$.
    % \COMMENT{so that $BA_{t-1}$ is updated in the direction $\widehat U_t$}
    \STATE $W_{t+1} \gets W_{t} - \eta \widehat G_t$
  \ENDFOR
  \STATE \textbf{Output:} $W_T$.
\end{algorithmic}
\end{algorithm}
