# Supplementary material for: LoRA and Privacy: When Random Projections Help (and When They Don't)
Source: arXiv:2601.21719 source file (2026-01-29)
Supplement: Supplementary file 3 [file projected_gradient_descent.tex]

\begin{algorithm}[H]
    \caption{Projection Gradient Descent \citet{kasiviswanathan21a}}\label{algo:proj-grad-desc}
    \textbf{Input:} Input dataset $D = (z_1, \dots, z_n)$, privacy parameters $(\varepsilon, \delta)$, learning rates $\{ \eta_t\}$, projection dimension parameters $\{\beta_t\}$.
    \begin{algorithmic}
    \STATE pick $w_1$ as any point in $\cC$
    \STATE \FOR{$t=1$ to $T$ do}
        \STATE Set $r_t \gets \min\{ d, c \cdot \omega(\cC)^2/\beta_t^2 \}$
        \STATE Let $\Phi_t \in \mathbb{R}^{r \times d} \sim_{i.i.d.} \mathcal{N}(0, 1/r_t)$
        \STATE Set $\sigma^2 \leftarrow \dfrac{32L^2T \log(1/\delta)}{n^2\epsilon^2}$
        \STATE Let $s_t \leftarrow \dfrac{\|\nabla F(\mathbf{w}_t;D)\|}{\|Z^\top \nabla F(\mathbf{w}_t;D)\|}$
        \STATE Let $\theta_t \leftarrow \Pi_{\Phi_t C}\!\Bigl(\Phi_t \mathbf{w}_t
      - \eta_t\bigl(s_t \Phi_t \nabla F(\mathbf{w}_t;D)+\mathbf{e}\bigr)\Bigr)$
      where $\mathbf{e}\sim \mathcal{N}(0,\sigma^2\mathbb{I}_m)$ 
        \STATE Let $\mathbf{w}_{t+1} \leftarrow$ pick any element from the set
      $S_t=\{\mathbf{w}\in C:\ \Phi_t\mathbf{w}=\theta_t\}$
    \ENDFOR        
    \end{algorithmic}
\end{algorithm}

We want to analyse this algorithm in our setting so that we can compare it to our results. So let's assume we are solving an unconstrained optimization problem (i.e. $\cC = \mathbb{R}^{d \times d}$) then we can drop the projection $\Pi_{Z^\top C}$ in the algorithm. Further $\Phi_t$ is exactly our $Z^\top$. However, the last step of picking an element in $S_t = \{ w \in \mathbb{R}^{d \times d}: Z^\top w = \theta_t\}$ is not exactly equal to multiplying with $Z$ as we do in our case, because $Z$ does not have orthonormal columns. However we can write the last step (going from $\theta_t$ to $w_t$) as matrix multiplication by setting $w_{t} = Q \theta_t$ where $Q = (Z^\top)^\dagger$ (the pseudoinverse). This means we can write the algorithm as 

\begin{algorithm}[H]
    \caption{Projection Gradient Descent \citet{kasiviswanathan21a}}\label{algo:proj-grad-desc}
    \textbf{Input:} Input dataset $D = (z_1, \dots, z_n)$, privacy parameters $(\varepsilon, \delta)$, learning rates $\{ \eta_t\}$, projection dimension parameters $\{\beta_t\}$.
    \begin{algorithmic}
    \STATE pick $w_1$ as any point in $\cC$
    \STATE \FOR{$t=1$ to $T$ do}
        \STATE Set $r_t \gets \min\{ d, c \cdot \omega(\cC)^2/\beta_t^2 \}$
        \STATE Let $Z^\top \in \mathbb{R}^{r \times d} \sim_{i.i.d.} \mathcal{N}(0, 1/r_t)$
        \STATE Set $\sigma^2 \leftarrow \dfrac{32L^2T \log(1/\delta)}{n^2\epsilon^2}$
        \STATE Let $s_t \leftarrow \dfrac{\|\nabla F(\mathbf{w}_t;D)\|}{\|Z^\top \nabla F(\mathbf{w}_t;D)\|}$
        \STATE Let $\theta_t \leftarrow Z^\top \mathbf{w}_t
      - \eta_t\bigl(s_t Z^\top \nabla F(\mathbf{w}_t;D)+\mathbf{e}\bigr)$
      where $\mathbf{e}\sim \mathcal{N}(0,\sigma^2\mathbb{I}_m)$ 
        \STATE Let $\mathbf{w}_{t+1} \leftarrow (Z^\top)^\dagger \theta_t$ 
    \ENDFOR        
    \end{algorithmic}
\end{algorithm}

Note that if we choose $Z \in \mathbb{R}^{d \times r}$ as an orthonormal matrix then $(Z^\top)^\dagger = Z$. So the question arises if we can do a similar analysis as in~\Cref{subsec:matproj-small-r} for $Z = SVD(X)$ where $X \in \mathbb{R}^{d \times r}$ with i.i.d coordinates dram from $\cN(0,1/r).$

% The question arises on how large to choose $\beta$, typically you would choose $\beta$ large enough so that with high probability we do not clip in order to preserve utility. As shown above we have that 
% \[
%     \frac{\partial \mathcal{L}}{\partial B} = \nabla_{W} \mathcal{L}(y)|_{W_t} A^\top
% \]
% and we recall that $A \in \mathbb{R}^{d \times r}$ is a Gaussian random matrix with i.i.d. coordinates sampled form $\cN(0, 1/r)$, therefore we have that 
% \[
%  \| \nabla_{W} \mathcal{L}(y)|_{W_t} A^\top \|_F^2   = \frac{1}{r} \sum_{i=1}^r a_i^\top ( \nabla_{W} \mathcal{L}(y)|_{W_t} \nabla_{W} \mathcal{L}(y)|_{W_t}^\top ) a_i
% \]
% where $a_i \in \mathbb{R}^d$ are i.i.d $\cN(0, \mathbf{I}_d)$. So 
% \[
%     \mathbb{E}[ \| \nabla_{W} \mathcal{L}(y)|_{W_t} A^\top \|_F^2 | V]= \text{tr}(\nabla_{W} \mathcal{L}(y)|_{W_t} \nabla_{W} \mathcal{L}(y)|_{W_t}^\top) = \| \nabla_{W} \mathcal{L}(y)|_{W_t}\|_F^2
% \]
% This means we need to choose the clipping threshold $ \beta\approx  \| \nabla_{W} \mathcal{L}(y)|_{W_t}\|_F$. 

% Therefore if we assume a bound $\beta$ on $\sum_{i=1}^T\nabla_{W} \mathcal{L}(y)|_{W_t} ^\top$ (as we would also do in the naive case) we directly obtain that the mechanism is DP by~\Cref{thm:matrix-dp-proj-mechanism-small-r}. And as illustrated in Figure (TO ADD) and~\Cref{cor:small-r-delta-improvement} we obtain that for $r$ small we obtain better privacy parameters for the same amount of noise, or equivalently need to add less noise to obtain the same privacy parameters.
